# Supplementary material for: Protected quasi-locality in quantum systems with long-range interactions
Source: arXiv:1503.01786 source file (2015-10-23)
Supplement: Supplementary file 1 [file suppmat.pdf]

# –*Supplemental Material*–
# Protected quasi-locality in quantum systems with long-range interactions

Lorenzo Cevolani,[1] Giuseppe Carleo,[1] and Laurent Sanchez-Palencia[1]

[1]*Laboratoire Charles Fabry, Institut d'Optique, CNRS, Univ. Paris Sud 11, 2 avenue Augustin Fresnel, F-91127 Palaiseau cedex, France*

In this Supplemental Material we give additional details on the methods and the analysis we have performed in the main Paper. In particular we provide a description of the time-dependent variational Monte Carlo method (Sec. I) and a microscopic derivation of the quasi-particle picture for both the long-range Ising and the long-range Bose-Hubbard models (Sec. II).

PACS numbers:

## I. TIME-DEPENDENT VARIATIONAL MONTE CARLO

We consider the unitary dynamics of lattice systems with long-range interactions after a quantum quench in the interaction strength is realized. In order to obtain an accurate description of the dynamics, we treat the time evolution by means of the time-dependent variational Monte Carlo (t-VMC) method [1]. This method is a general framework to obtain the optimal time evolution of a given variational state, which is conveniently parametrized as

$$\Psi(\mathbf{X},t) \;=\; \exp\left[\sum_k \alpha_k(t)\mathcal{O}_k(\mathbf{X})\right]\times\Phi(\mathbf{X}), \qquad (1)$$

where $\mathbf{X}$ is a given many-body basis on which the wave-function is projected, $\alpha_i$ is a set of complex-valued variational parameters, $\mathcal{O}_k(\mathbf{X}) = \frac{1}{\Psi(\mathbf{X},t)}\frac{\partial\Psi(\mathbf{X},t)}{\partial\alpha_k(\mathbf{X})}$, and $\Phi(\mathbf{X})$ is some time-independent state.

By means of the Dirac-Frenkel time-dependent variational principle, it can be shown that the optimal variational parameters have to satisfy, at each time, the following equations of motion

$$i\sum_{k'}\langle\mathcal{O}_k^\star\mathcal{O}_{k'}\rangle_t^{\mathrm{c}}\,\dot{\alpha}_{k'}(t) \;=\; \langle\mathcal{O}_k^\star\mathcal{H}\rangle_t^{\mathrm{c}}, \qquad (2)$$

where $\mathcal{H}$ is the system hamiltonian, $\langle AB\rangle_t^{\mathrm{c}} \equiv \langle AB\rangle_t - \langle A\rangle_t\langle B\rangle_t$ are two-point connected averages, and $\langle\dots\rangle_t \equiv \frac{\langle\Psi(t)|\dots|\Psi(t)\rangle}{\langle\Psi(t)|\Psi(t)\rangle}$ denote expectation values over the variational state at time $t$.

Since the variational state is typically taken to be non-locally entangled, the former expectation values cannot be computed exactly with the approaches used, for example, within Matrix Product States techniques. The expectation values are therefore obtained from Monte Carlo sampling of the (sign-problem-free) square modulus of the variational wave-function, and the equations of motion (2) are then solved.

The t-VMC approach has been so-far used to simulate the dynamics of both one and two-dimensional lattice systems [1, 2]. In general, with a sensible choice of the variational states, it allows to simulate both the short and the long-time dynamics of correlated quantum systems with an accuracy comparable to methods based on tensor-network variational states.

### A. Jastrow states for spins and bosons

For the lattice systems studied here, we consider time-evolved wave-functions of the general form given by the Jastrow-Feenberg (JF) correlations expansion,

$$\Psi_{\mathrm{JF}}(\mathbf{X},t) = \exp\Bigg[\sum_i J_i^{(1)}(t)\mathcal{D}_i + \frac{1}{2}\sum_{i,j}J_{ij}^{(2)}(t)\mathcal{D}_i\mathcal{D}_j + \\ + \frac{1}{3!}\sum_{ijk}J_{ijk}^{(3)}(t)\mathcal{D}_i\mathcal{D}_j\mathcal{D}_k + \dots\Bigg]\times\Phi(\mathbf{X}), \qquad (3)$$

where the time-dependent variational parameters are the complex amplitudes of the $m$-body Jastrow tensors $J^{(m)}_{i_1 i_2\dots i_m}(t)$, $\mathcal{D} = \{\mathcal{D}_1(\mathbf{X}),\mathcal{D}_2(\mathbf{X})\dots D_L(\mathbf{X})\}$ is the set of $L$ operators in which the expansion is performed, and $\Phi(\mathbf{X})$ is a time-independent state solution of the non-interacting problem. This expansion accurately describes equilibrium properties of a variety of prototypical correlated quantum systems. It provides an accurate description of the Mott transition both in the bosonic and fermionic Hubbard models [3], and of the equilibrium properties of superfluid Helium 4 [4], to name a few classical references. Moreover, it can be shown that an ansatz containing only up to the second order correlation tensor is an exact description of important prototypical models, both with short-range (Luttinger liquids) [5] and long-range (Calogero-Sutherland) interactions [6].

For spin Hamiltonians, we consider an expansion in the local spin operators, i.e. $\mathcal{D}_{\mathrm{LRTI}} = (\sigma_1^z,\dots\sigma_L^z)$. In this case the non-interacting state is taken to be a mere constant. For bosonic systems, the JF expansion is performed in the density operators, namely $\mathcal{D}_{\mathrm{LRBH}} = (n_1,\dots n_L)$, therefore systematically including high-order density-density correlations in the wave-function. In this latter case the non-interacting state is taken to be the

superfluid state in the absence of interactions. In both cases, due to the homogeneity and the translation invariance of the system, we have $J_i^{(1)} = 0$ and $J_{i,j}^{(2)} = J_{|i-j|}^{(2)}$.

For the quantum quenches we consider here, where the system is prepared in relatively weakly interacting initial states, we have checked that the inclusion of 3-body and higher terms in the JF expansion doesn't change quantitatively our conclusions on the locality behavior. In the main Paper we therefore present results where the JF expansion includes up to 2-body tensors.

## II. QUASI-PARTICLE APPROACH

In our Paper we consider two types of system: a bosonic and a spin one. Even if their Hamiltonians are of different nature, we will show in the following that both of them can be reduced, in specific regimes, in the following general form

$$\mathcal{H} = \frac{1}{2}\sum_k \left[\mathcal{A}_k \left(b_k^\dagger b_k + b_{-k} b_{-k}^\dagger\right) + \mathcal{B}_k \left(b_k^\dagger b_{-k}^\dagger + b_{-k} b_k\right)\right], \quad (4)$$

where the quantities $\mathcal{A}_k$ and $\mathcal{B}_k$ are real-valued even functions of $k$, and the $b_k(b_k^\dagger)$ are bosonic annihilation (creation) operators. Using a matrix representation where $V_k^\dagger = \begin{pmatrix} b_k^\dagger & b_{-k} \end{pmatrix}$ and $\mathbb{M}_k = \begin{pmatrix} \mathcal{A}_k & \mathcal{B}_k \\ \mathcal{B}_k & \mathcal{A}_k \end{pmatrix}$, the Hamiltonian reads

$$\mathcal{H} = \frac{1}{2}\sum_k V_k^\dagger \mathbb{M}_k V_k.$$

This Hamiltonian can be diagonalized with the standard transformation $V_k = \mathbb{A}_k W_k$ where $W_k^\dagger = \begin{pmatrix} \beta_k^\dagger & \beta_{-k} \end{pmatrix}$ is the vector composed by Bogoliubov quasi-particles, the matrix $\mathbb{A}_k = \begin{pmatrix} u_k & v_k \\ v_k & u_k \end{pmatrix}$ diagonalizes $\mathbb{M}_k$ and it has $\det \mathbb{A}_k = 1$. These last two conditions are sufficient to determine the coefficients:

$$\begin{aligned} u_k &= \sqrt{\frac{1}{2}\left(\mathcal{A}_k/\sqrt{\mathcal{A}_k^2 - \mathcal{B}_k^2} + 1\right)}, \\ v_k &= -\text{sign}(\mathcal{B}_k)\sqrt{\frac{1}{2}\left(\mathcal{A}_k/\sqrt{\mathcal{A}_k^2 - \mathcal{B}_k^2} - 1\right)}. \end{aligned}$$

To study the out-of-equilibrium dynamics we assume that the system is prepared in the ground state of an initial Hamiltonian defined by $\mathbb{M}_k^i$ and that a sudden change, a quantum quench, is performed in this matrix to a final matrix $\mathbb{M}_k^f$. This change induces a non-trivial time evolution of the particle operators $b_k(t)$. The natural basis to study this evolution is that of $V_k = \mathbb{A}_k^f W_k^f$, since in this basis the final Hamiltonian is diagonal, $\mathcal{H}_f = \sum_k E_k^f \beta_k^{f\dagger} \beta_k^f$. The dispersion relation of the quasi-particles in the final basis is

$$E_k^f = \sqrt{\mathcal{A}_k^2 - \mathcal{B}_k^2} \quad (5)$$

and the time evolution of the quasi-particle operator is $\beta_k^f(t) = \mathrm{e}^{-iE_k^f t}\beta_k^f(0)$. At time $t = 0$ the operators $b_k$ can be expanded on both the initial and final bases $V_k = \mathbb{A}_k^i W_k^i = \mathbb{A}_k^f W_k^f$. It yields a linear relation between pre- and post-quench operators, $W_k^f = \left(\mathbb{A}_k^f\right)^{-1} \mathbb{A}_k^i W_k^i$. This relation is useful because we know that $W_k^i$ acts trivially on the initial state, the ground state of the initial Hamiltonian, namely $\beta_k^i|0\rangle = 0$.

We can use the previous relations to compute the time evolution of some observables. We will focus on observables that are quadratic in the particles operators, for example the $\langle n_i(t) n_j(t)\rangle$ correlation function in the LRBH model and the $\langle \sigma_i^z(t)\sigma_j^z(t)\rangle$ in the LRTI model. One of the most general, real quadratic operators that conserve the translational invariance of the system and the particles number takes the form

$$\begin{aligned} g(R;t) = \frac{1}{N}\sum_k e^{-ikR}\big(&\langle b_k^\dagger b_k\rangle + \langle b_{-k} b_{-k}^\dagger\rangle + \\ &+ \langle b_{-k} b_k\rangle + \langle b_k^\dagger b_{-k}^\dagger\rangle\big) \quad (6) \end{aligned}$$

where the expectation value is taken over the initial ground state $|0\rangle$. The time evolution is due to the operators $\alpha_k^f$ and it involves only the final dispersion relation $E_k^f$, namely $2E_k^f$ because $b_k^\dagger b_k$ is the product of two $\beta_k(t)$ and $\beta_k^\dagger(t)$. The amplitude of oscillations is given by the transformation between pre- and post- quench operators $\beta_k^i(0)$ and $\beta_k^f(0)$ that depends on all the coefficients $\mathcal{A}_k^i$, $\mathcal{B}_k^i$, $\mathcal{A}_k^f$ and $\mathcal{B}_k^f$. We then find:

$$\begin{aligned} g(R,t) - g(R,0) = \int_{-\pi}^{+\pi} \frac{dk}{2\pi} \cos(kR) \times \\ \times \left[\frac{\mathcal{A}_k^i \mathcal{B}_k^f - \mathcal{A}_k^f \mathcal{B}_k^i}{E_k^i\left(\mathcal{A}_k^f + \mathcal{B}_k^f\right)}\right] \times \left[1 - \cos\left(2E_k^f t\right)\right], \end{aligned}$$

which is Eq. (3) of the main Paper with:

$$\mathcal{F}(k) = \frac{\mathcal{A}_k^i \mathcal{B}_k^f - \mathcal{A}_k^f \mathcal{B}_k^i}{E_k^i\left(\mathcal{A}_k^f + \mathcal{B}_k^f\right)}.$$

Note that we can see a time dependent part, that goes to zero as $1/\sqrt{t}$ for large $t$, as predicted by the stationary phase argument, and the time independent part which is the thermalization value.

### A. Long-Range Transverse Ising model

We first study the long-range transverse Ising chain (LRTI), the Hamiltonian of which reads

$$\mathcal{H}_{LRTI} = -h\sum_i \sigma_i^x + \frac{V}{2}\sum_{i\neq j}\frac{\sigma_i^z\sigma_j^z}{|i-j|^\alpha}.$$

Close to a polarized phase, this Hamiltonian can be written in the form of Eq. 4 using linear spin wave theory (LSWT). We first replace the spin operators by classical spins $S_i^\alpha = \frac{1}{2}\sigma_i^\alpha$. Then, we find the minimum of the classical energy rotating the reference frame around the $y$ axis with an angle $\gamma$, $S_i' = \mathcal{R}_i(\gamma)S_i$. As a function of the rotated spin operators the Hamiltonian reads

$$\begin{aligned}\mathcal{H}_{LRTI} = 2V\sum_{i\neq j}\frac{1}{|i-j|^\alpha}\left[\cos^2(\gamma)\,S_i^{z\prime}S_j^{z\prime} + \sin^2(\gamma)\,S_i^{x\prime}S_j^{x\prime} + \right.\\ \left. -\sin(\gamma)\cos(\gamma)\left(S_i^{z\prime}S_j^{x\prime} + S_i^{x\prime}S_j^{z\prime}\right)\right] + \\ + 2h\sum_i\left(\sin(\gamma)\,S_i^{z\prime} + \cos(\gamma)\,S_i^{x\prime}\right).\end{aligned}$$

In order to introduce bosonic operators, we use the Holstein-Primakoff transformations for spin one-half, $S_i^{z\prime} \approx \frac{1}{2}\left(b_i^\dagger + b_i\right)$, $S_i^{x\prime} = b_i^\dagger b_i - \frac{1}{2}$ and treat the Hamiltonian perturbatively in the $b_i$ operators. The zero order term is the classical energy per particle, $E_{cl} = \left[\frac{V}{2}\sin^2(\gamma)\,\bar{P} + h\cos(\gamma)\right]$, where $\bar{P} = \sum_{R>0} 1/R^\alpha$ is the average interaction energy. We fix the rotation angle $\gamma$ imposing the minimum of the classical energy. In the case of a quasi-classical state, $V \ll h$, the minimum corresponds to $\gamma = 0$ and we will use this value to simplify our expressions. The linear term in the $b_i$ operators vanishes on the minimum of the classical energy. Then the quantum corrections appear at quadratic order, that in momentum space reads

$$\begin{aligned}\mathcal{H}_{LRTI} - NE_{cl} = \frac{1}{2}\sum_k\left[\left(b_k^\dagger b_k + b_{-k}b_{-k}^\dagger\right)(VP(k) + 2h) + \right.\\ \left. + VP(k)\left(b_k^\dagger b_{-k}^\dagger + b_{-k}b_k\right)\right],\end{aligned}$$

where $P(k)$ is the Fourier transform of the long-range potential and the quasi-particle energy is

$$E_k = 2\sqrt{h(h + VP(k))}.$$

Note that the latter is well behaved for $V \ll h$, where our expressions hold.

In the main Paper we consider the correlations along the $z$-axis, which reads $G(R,t) = \langle\sigma_i^z\sigma_j^z\rangle$, in real space. Using the Holstein-Primakoff transformation it becomes $G(R,t) = \langle\left(b_i^\dagger + b_i\right)\left(b_j^\dagger + b_j\right)\rangle$, in terms of bosonic operators, which is exactly Eq. 6 in real space. Taking the Fourier transform we get $G(R,t) - G(R,0) = g(R,t)$. The main parameters in the LRTI model are

$$\begin{aligned}\mathcal{A}_k &= VP(k) + 2h\\ B_k &= VP(k)\\ \mathcal{F}^{\sigma\sigma}(k) &= 2\,\frac{(h_f V_i - h_i V_f)\,P(k)}{(h_f + V_f P(k))\,E_k^i}.\end{aligned}$$

Setting $h_i = h_f = 1$ we find the same expression found in the Paper.

### B. Long-Range Bose-Hubbard model

For the long-range Bose-Hubbard Hamiltonian we can write the Hamiltonian directly in Fourier space as

$$\mathcal{H}_{LRBH} = \sum_k \epsilon_k b_k^\dagger b_k + \frac{1}{2L}\sum_{k,p,q} V(q) b_{k-q}^\dagger b_{p+q}^\dagger b_p b_k,$$

in the standard second quantization form, where $\epsilon_k = 4J\sin^2\left(\frac{k}{2}\right)$ is the usual dispersion for the free lattice system. The Fourier transform of the potential is $V(q) = U + VP(q)$ where $U$ is the on-site short-range interaction strength, $V$ is the long-range interaction strength and $P(q)$ its the Fourier transform with the regularization condition $P(q=0) = 0$. Since the $k=0$ component are macroscopically populated we can separate them from the other momenta and take this expansion up to the second order in $b_0$ and $b_0^\dagger$. It yields

$$\begin{aligned}\mathcal{H}_{LRBH} \approx \frac{V(0)}{2L} b_0^\dagger b_0^\dagger b_0 b_0 + \sum_{k\neq 0}\epsilon_k b_k^\dagger b_k + \\ + \frac{n_0}{2L}\sum_{k\neq 0}\left\{2\left[V(k) + V(0)\right] b_k^\dagger b_k + b_k^\dagger b_{-k}^\dagger + b_{-k}b_k\right\},\end{aligned}$$

using the relation $\left(b_0^\dagger b_0\right)^2 \approx N^2 - 2N\sum_{k\neq 0} b_k^\dagger b_k$ and we get, up to a constant, the Hamiltonian

$$\begin{aligned}\mathcal{H}_{LRBH} = \frac{1}{2}\sum_{k\neq 0}\left[\left(b_k^\dagger b_k + b_{-k}b_{-k}^\dagger\right)(\epsilon_k + n_0 V(k)) + \right.\\ \left. + n_0 V(k)\left(b_k^\dagger b_{-k}^\dagger + b_{-k}b_k\right)\right],\end{aligned}$$

where $n_0$ is the condensate fraction. In this case we can therefore identify $\mathcal{A}_k = \epsilon_k + n_0 V(k)$ and $\mathcal{B}_k = n_0 V(k)$. Inserting these expressions into Eq. 5, we then find the dispersion relation of the quasi-particles $E_k = \sqrt{\epsilon_k\left(\epsilon_k + 2n_0 V(k)\right)}$.

In the LRBH case, we consider the density-density correlations, $G(R;t) = \langle n_i(t) n_j(t)\rangle = \frac{1}{N}\sum_k \mathrm{e}^{-\imath kR}\langle n_k(t) n_{-k}(t)\rangle$, where we have introduced the Fourier transform of the density $n_k(t) = \sum_q b_{k+q}^\dagger b_q$. Using the Bogoliubov expansion in powers of the $k=0$ mode, we write the correlation in the form of Eq. 6, namely $G(R,t) - G(R,0) = n_0 g(R,t)$. Hence the main

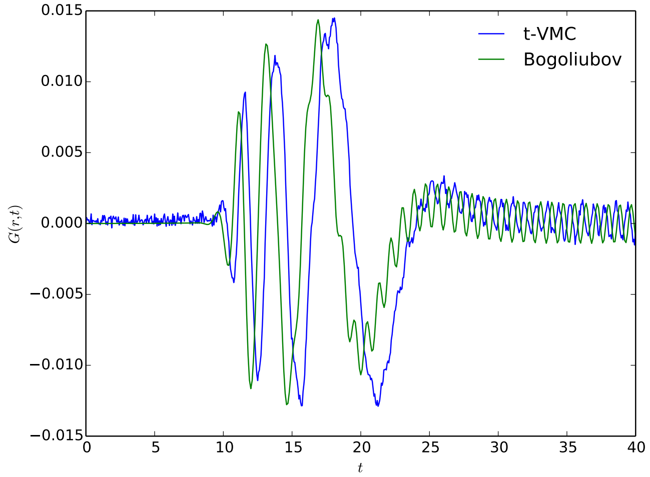


FIG. 1: Comparison between the density-density correlations obtained with the t-VMC approach (with the inclusion of the 2-body tensor, blue curve) and the Bogoliubov analysis (green curve) for $\alpha = 3, V_i = U_i = 1$, and $V_f = U_f = \frac{1}{4}$. Here the distance is $R = 40$.

parameters of the LRBH model are

$$\begin{aligned} \mathcal{A}_k &= \epsilon_k + n_0 V(k) \\ \mathcal{B}_k &= n_0 V(k) \\ E_k &= \sqrt{\epsilon_k \left(\epsilon_k + 2n_0 V(k)\right)} \\ \mathcal{F}^{nn}(k) &= n_0^2 \frac{\epsilon_k \left(V_i(k) - V_f(k)\right)}{E_k^i \left(\epsilon_k + 2n_0 V_f(k)\right)}. \end{aligned}$$

In the case $U_i = U_f$ we get the expression given in the Paper.

### C. Validity of the quasi-particle picture

In the main Paper we use the quasi-particle picture, in order to interpret the various dynamical regimes we have observed in the many-body correlations. This picture is based on the assumption that, after a quantum quench, freely-propagating quasi-particles are released, whose interactions can be neglected. The quasi-particle picture can legitimately be questioned on the basis that it neglects weak residual interactions between the quasi-particles. In order to test the validity of the quasi-particle picture, we have systematically compared the space-time behavior of the correlation functions given by the quasi-particle and many-body t-VMC approaches.

In Fig. 1 we show a direct comparison of the time-dependent density-density correlations for the LRBH model. The two approaches (t-VMC on one hand and Bogoliubov analysis on the other hand) yield quantitatively similar results. The slight discrepancy is here due to a renormalized quasi-particle velocity in the correlated t-VMC approach, which results in slightly faster propagating signals. More precisely we have determined the cone velocities given by the two approaches in Table I. We find that the quasi-particle and many-body t-VMC approaches give very close values with a discrepancy of the order of 4%. This legitimates the quasi-particle picture for all values of $\alpha$.

| LRTI | $\alpha = 3$ | LRBH | $\alpha = 1/2$ | $\alpha = 3/2$ | $\alpha = 3$ |
|---|---|---|---|---|---|
| $v_c^{\text{t-VMC}}$ | $0.37\,h$ | $v_c^{\text{t-VMC}}$ | $3.6\,J$ | $3.5\,J$ | $3.1\,J$ |
| $v_c^{\text{qp}}$ | $0.393\,h$ | $v_c^{\text{qp}}$ | $3.740\,J$ | $3.389\,J$ | $3.177\,J$ |

TABLE I: Comparison of the cone velocities obtained from both the t-VMC method and the quasi-particle picture. The t-VMC velocities are obtained as a fit of the activation time $vt^\star = R$ (see main Paper), with a statistical uncertainty of $\sim \pm 0.01\,h$ (for the LRTI model) and $\sim \pm 0.1\,J$ (for the LRBH model). The reported $v_c^{\text{qp}}$ equals twice the maximum group velocity of the quasi-particles, i.e. $v_c^{\text{qp}} = 2 \times \max_k \partial_k E_k$.

In general, in the regime that precedes the arrival of the correlation front the scattering processes between the fastest traveling quasi-particles are to all purposes negligible, and the ballistic spreading is a direct consequence of this. Therefore, because of the almost non-interacting nature of the quasi-particles in the ballistic regime, the Bogoliubov dynamics captures qualitatively well the correlation front. Nevertheless, the picture of independent quasi-particles inevitably breaks down on time scales $t \gg t^\star$ when scattering processes coupling all the excited modes play a key role in the decay of the correlation function. We have indeed found regimes, for interactions significantly stronger than those studied in the Paper, where at large times the damping of the signal is substantially different between the t-VMC and the Bogoliubov approach.

For what concerns the LRTI model, the agreement between t-VMC and the simple LSW theory is less accurate than Bogoliubov theory for the LRBH model. This has been already observed in Ref [7]. We believe that the origin of the quantitative discrepancy is due to the order retained in the Holstein-Primakoff transformation, which effectively amounts to treat hard-core bosons as if they were soft-core bosons. This approximation is certainly crude in this case and breaks the full quantitative agreement. However, we conclude stressing that the qualitative features are still reproduced in a fair way.

Most important, we find that the correlation front studied in the Paper fairly reproduced by the LSW theory. As shown in Table I, the cone velocity given by the LSW theory is in good agreement with that of the many-body t-VMC approach in the ballistic regime ($\alpha = 3$).

[1] G. Carleo, F. Becca, M. Schiró, and M. Fabrizio, Sci. Rep. **2**, 243 (2012).
[2] G. Carleo, F. Becca, L. Sanchez-Palencia, S. Sorella, and M. Fabrizio, Phys. Rev. A **89**, 031602 (2014).
[3] M. Capello, F. Becca, M. Fabrizio, and S. Sorella, Phys. Rev. Lett. **99**, 056402 (2007).
[4] W. L. McMillan, Phys. Rev. **138**, A442 (1965).
[5] B. Tayo and S. Sorella, Phys. Rev. B **78**, 115117 (2008).
[6] B. Sutherland, *Beautiful Models* (World Scientific Publishing Company, 2004).
[7] P. Hauke and L. Tagliacozzo, Phys. Rev. Lett. **111**, 207202 (2013).
